# Supplementary material for: Signs of Language: Embodied Sign Language Fingerspelling Acquisition from Demonstrations for Human-Robot Interaction
Source: arXiv:2209.05135 source file (2023-06-05)
Supplement: Supplementary file 1 [file additional.tex]

\setcounter{figure}{0}

\setcounter{table}{0}

\section{Supplementary material}

\subsection{Controller tuning}

Figure~\ref{fig:controller100} illustrates the error value for values of $k_p$ and $k_d$ in the range [0, 100], Figure~\ref{fig:controller10} for [0, 10] and Figure~\ref{fig:controller1} for [0, 1].

\begin{figure*}[ht]
    \centering
    \begin{subfigure}{\textwidth}
        \centering
        \includegraphics[width=0.99\textwidth]{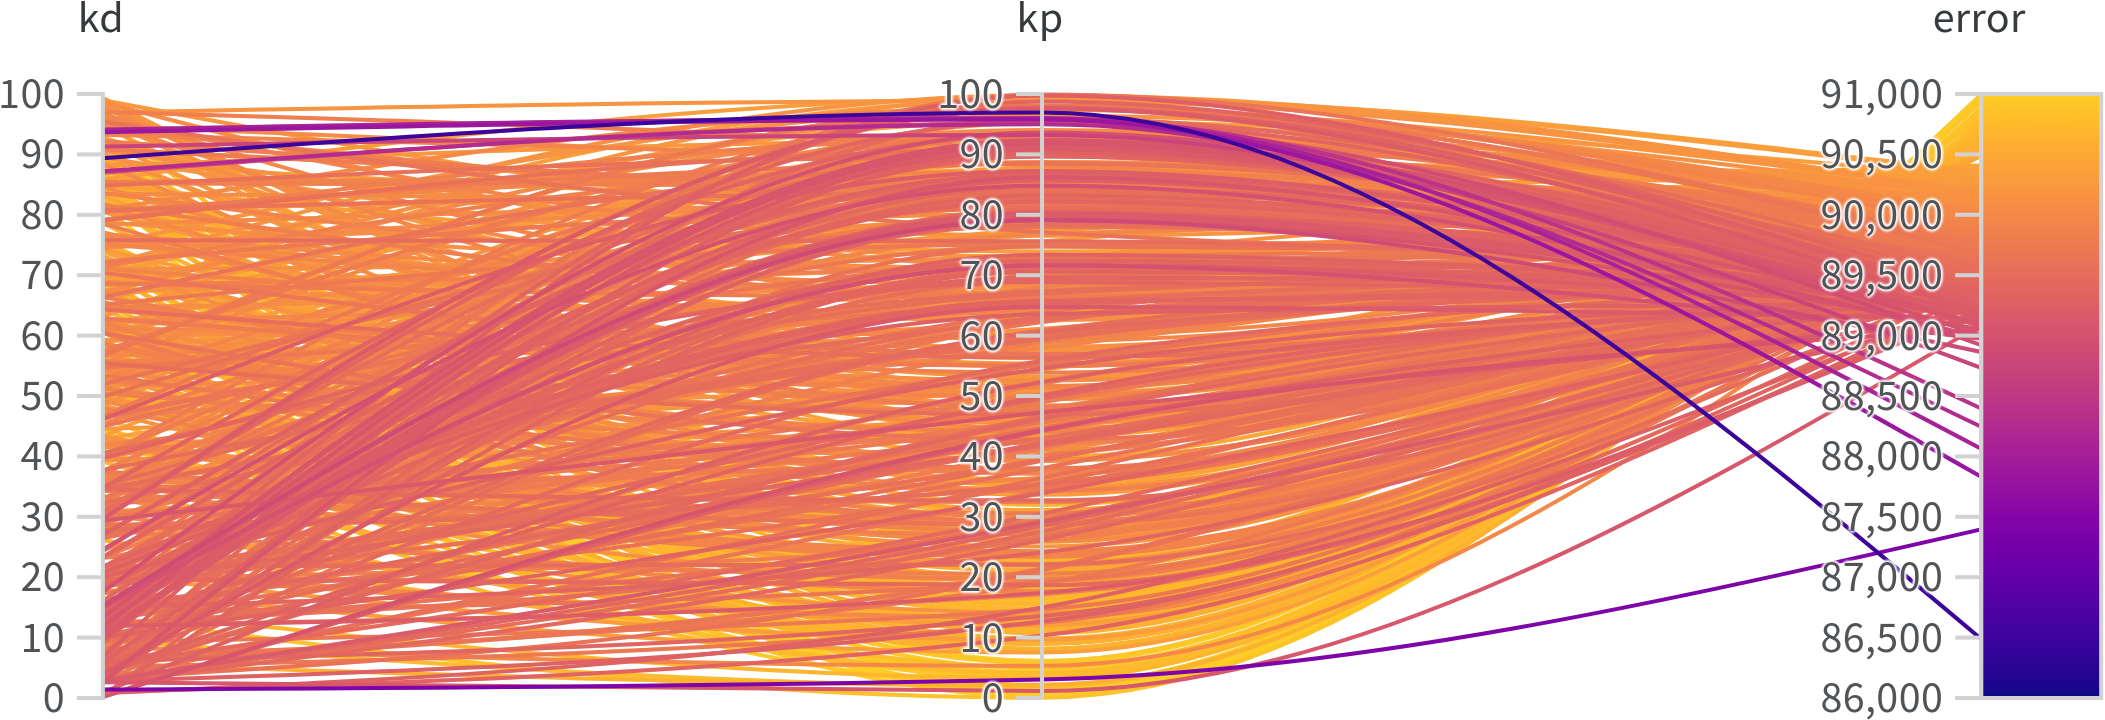}
        \caption{Max value 100}
        \label{fig:controller100}
    \end{subfigure}
    \vfill
    \begin{subfigure}{\textwidth}
        \centering
        \includegraphics[width=0.99\textwidth]{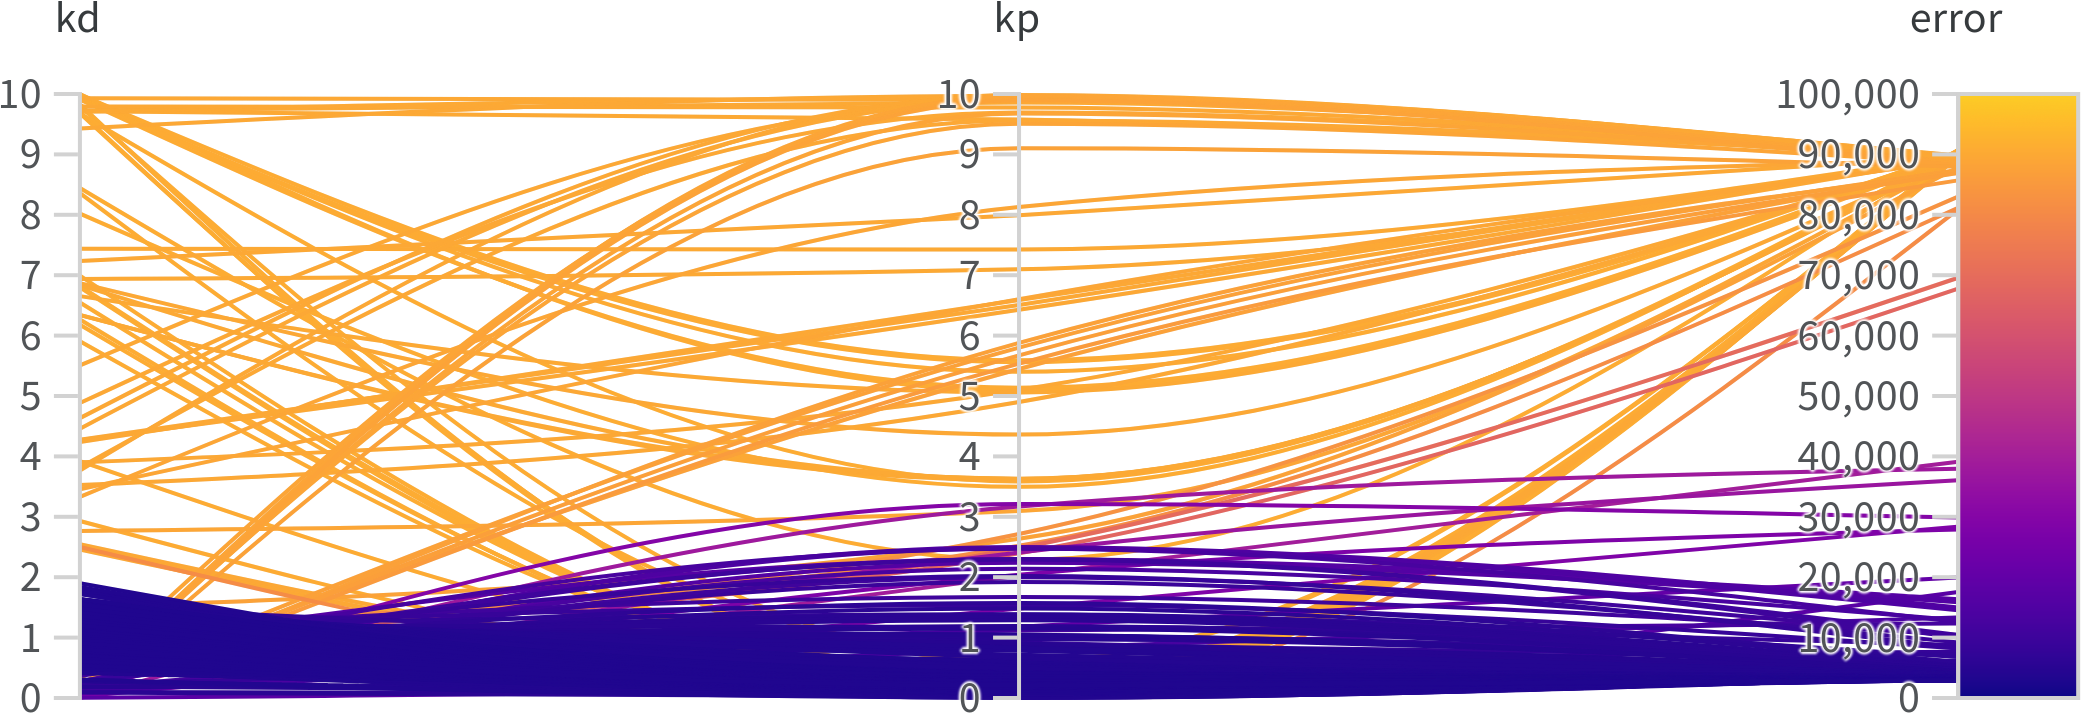}
        \caption{Max value 10}
        \label{fig:controller10}
    \end{subfigure}
    \vfill
    \begin{subfigure}{\textwidth}
        \centering
        \includegraphics[width=0.99\textwidth]{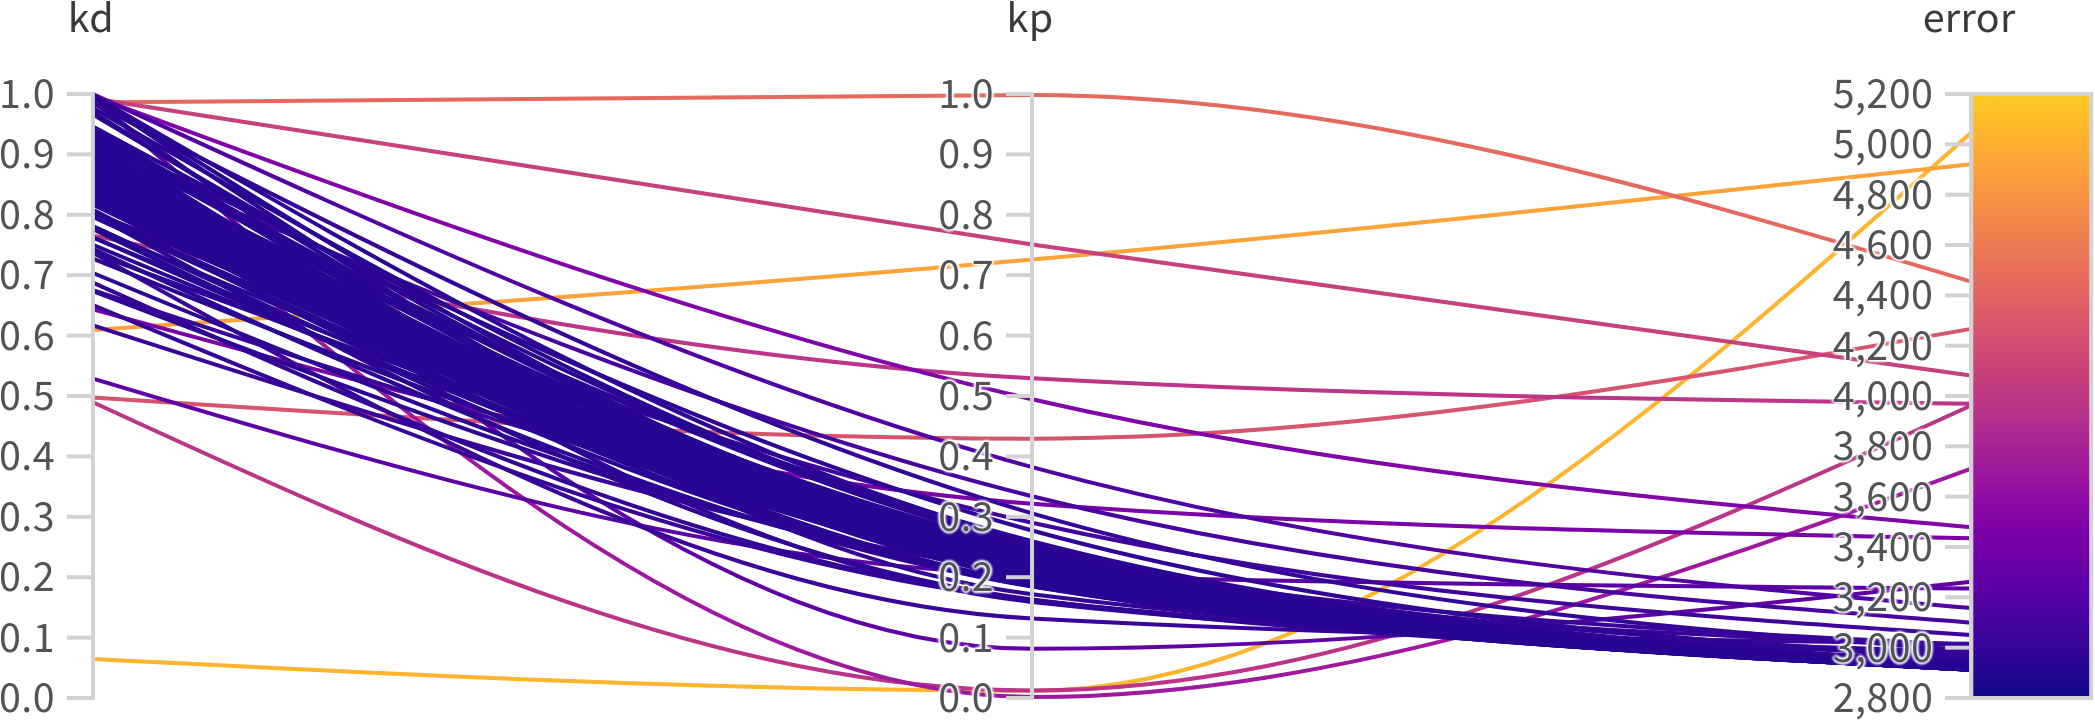}
        \caption{Max value 1}
        \label{fig:controller1}
    \end{subfigure}
    \caption{Exploration of different values of $k_p$ and $k_d$}
    \label{fig:controller_sweep}
\end{figure*}

\newpage

\subsection{Reinforcement learning tuning}

Table~\ref{tab:my-table} provides an alternative version of the results illustrated in Figure~\ref{fig:tuning} from the paper. The table is sorted in ascending order based on the reward. Complementarily, Figure~\ref{fig:corr} provides the correlation to the reward (i.e., last column and/or row) for each parameter. 

\begin{table}[ht]
\centering
\resizebox{\textwidth}{!}{%
\begin{tabular}{ccccccccc}
\hline \hline
\textbf{batch\_size} &
  \textbf{gamma} &
  \textbf{learning\_rate} &
  \textbf{log\_std\_init} &
  \textbf{n\_epochs} &
  \textbf{n\_steps} &
  \textbf{ortho\_init} &
  \textbf{weight\_decay} &
  \textbf{eval/mean\_reward} \\ \hline

128 & 0.9  & 0.00001  & -2 & 10 & 1024 & false & 0.00001 & 1624.15 \\
128 & 0.9  & 0.00001  & -2 & 10 & 512  & false & 0.00001 & 1585.71 \\
128 & 0.9  & 0.00001  & -1 & 10 & 1024 & false & 0.00001 & 1531.93 \\
128 & 0.9  & 0.00001  & -2 & 10 & 512  & true  & 0.00001 & 1523.36 \\
128 & 0.9  & 0.00001  & -1 & 10 & 512  & false & 0.00001 & 1482.61 \\
128 & 0.9  & 0.00001  & -2 & 5  & 512  & true  & 0.00001 & 1471.42 \\
128 & 0.9  & 0.00001  & -2 & 5  & 512  & false & 0.00001 & 1448.38 \\
128 & 0.9  & 0.00001  & -2 & 10 & 512  & true  & 0.00001 & 1443.02 \\
128 & 0.9  & 0.00001  & -2 & 5  & 512  & true  & 0.00001 & 1422.17 \\
256 & 0.9  & 0.00001  & -2 & 5  & 1024 & true  & 0.00001 & 1413.56 \\
128 & 0.9  & 0.00003  & -1 & 10 & 1024 & false & 0.0001  & 1389.84 \\
128 & 0.95 & 0.00001  & -1 & 10 & 512  & true  & 0.00001 & 1365.09 \\
128 & 0.9  & 0.00001  & -1 & 5  & 1024 & false & 0.00001 & 1365.08 \\
128 & 0.95 & 0.00001  & -1 & 10 & 512  & false & 0.00001 & 1345.54 \\
128 & 0.9  & 0.00001  & -2 & 5  & 1024 & true  & 0.00001 & 1328.81 \\
256 & 0.95 & 0.00001  & -1 & 10 & 1024 & false & 0.00001 & 1316.15 \\
128 & 0.95 & 0.00001  & -2 & 5  & 512  & true  & 0.00001 & 1314.80 \\
128 & 0.9  & 0.00003  & -1 & 10 & 1024 & false & 0.00001 & 1300.67 \\
128 & 0.95 & 0.00001  & -2 & 10 & 512  & true  & 0.00001 & 1297.27 \\
256 & 0.9  & 0.00001  & -1 & 10 & 512  & true  & 0.00001 & 1291.71 \\
128 & 0.9  & 0.00001  & -2 & 10 & 4096 & false & 0.00001 & 1280.08 \\
128 & 0.9  & 0.00003  & -2 & 10 & 1024 & true  & 0.00001 & 1260.49 \\
256 & 0.9  & 0.00001  & -1 & 5  & 1024 & true  & 0.00001 & 1246.09 \\
256 & 0.95 & 0.00001  & -1 & 10 & 1024 & true  & 0.0001  & 1235.01 \\
128 & 0.95 & 0.00001  & -1 & 10 & 1024 & true  & 0.00001 & 1210.89 \\
256 & 0.9  & 0.00001  & -1 & 10 & 1024 & true  & 0.00001 & 1202.36 \\
256 & 0.95 & 0.00003  & -2 & 10 & 512  & true  & 0.00001 & 1194.46 \\
128 & 0.95 & 0.00003  & -1 & 10 & 1024 & false & 0.00001 & 1124.79 \\
128 & 0.95 & 0.00001  & -2 & 10 & 1024 & false & 0.00001 & 1123.54 \\
128 & 0.9  & 0.00001  & -1 & 10 & 1024 & true  & 0.00001 & 1120.74 \\
256 & 0.9  & 0.000003 & -1 & 10 & 1024 & false & 0.00001 & 1079.17 \\
128 & 0.9  & 0.000001 & -2 & 10 & 1024 & true  & 0.00001 & 1072.54 \\
128 & 0.9  & 0.000001 & -3 & 5  & 512  & true  & 0.00001 & 1057.06 \\
128 & 0.9  & 0.00003  & -2 & 3  & 4096 & true  & 0.00001 & 1044.13 \\
128 & 0.95 & 0.000001 & -2 & 5  & 1024 & true  & 0.00001 & 1042.69 \\
128 & 0.9  & 0.000003 & -1 & 5  & 1024 & false & 0.00001 & 997.65  \\
256 & 0.9  & 0.000001 & -2 & 10 & 512  & false & 0.00001 & 958.96  \\
128 & 0.95 & 0.000001 & -1 & 10 & 1024 & false & 0.00001 & 930.24  \\
512 & 0.9  & 0.000003 & -3 & 3  & 4096 & true  & 0.00001 & 929.63  \\
128 & 0.9  & 0.00003  & -1 & 10 & 512  & false & 0.00001 & 922.81  \\
256 & 0.9  & 0.00003  & -2 & 5  & 1024 & true  & 0.00001 & 915.33  \\
128 & 0.95 & 0.000001 & -1 & 10 & 512  & false & 0.00001 & 898.50  \\
128 & 0.9  & 0.000001 & -1 & 10 & 512  & true  & 0.00001 & 893.27  \\
128 & 0.95 & 0.000001 & -1 & 5  & 512  & true  & 0.00001 & 883.68  \\
128 & 0.95 & 0.00003  & -2 & 5  & 4096 & false & 0.00001 & 870.71  \\
128 & 0.9  & 0.00001  & -3 & 10 & 1024 & false & 0.00001 & 854.40 \\ \hline \hline
\end{tabular}%
}
\caption{Hyperparameters combinations and relative results for the tuning based on the reference motion}
\label{tab:my-table}
\end{table}

\begin{figure*}[ht]
    \centering
    \includegraphics[width=\textwidth]{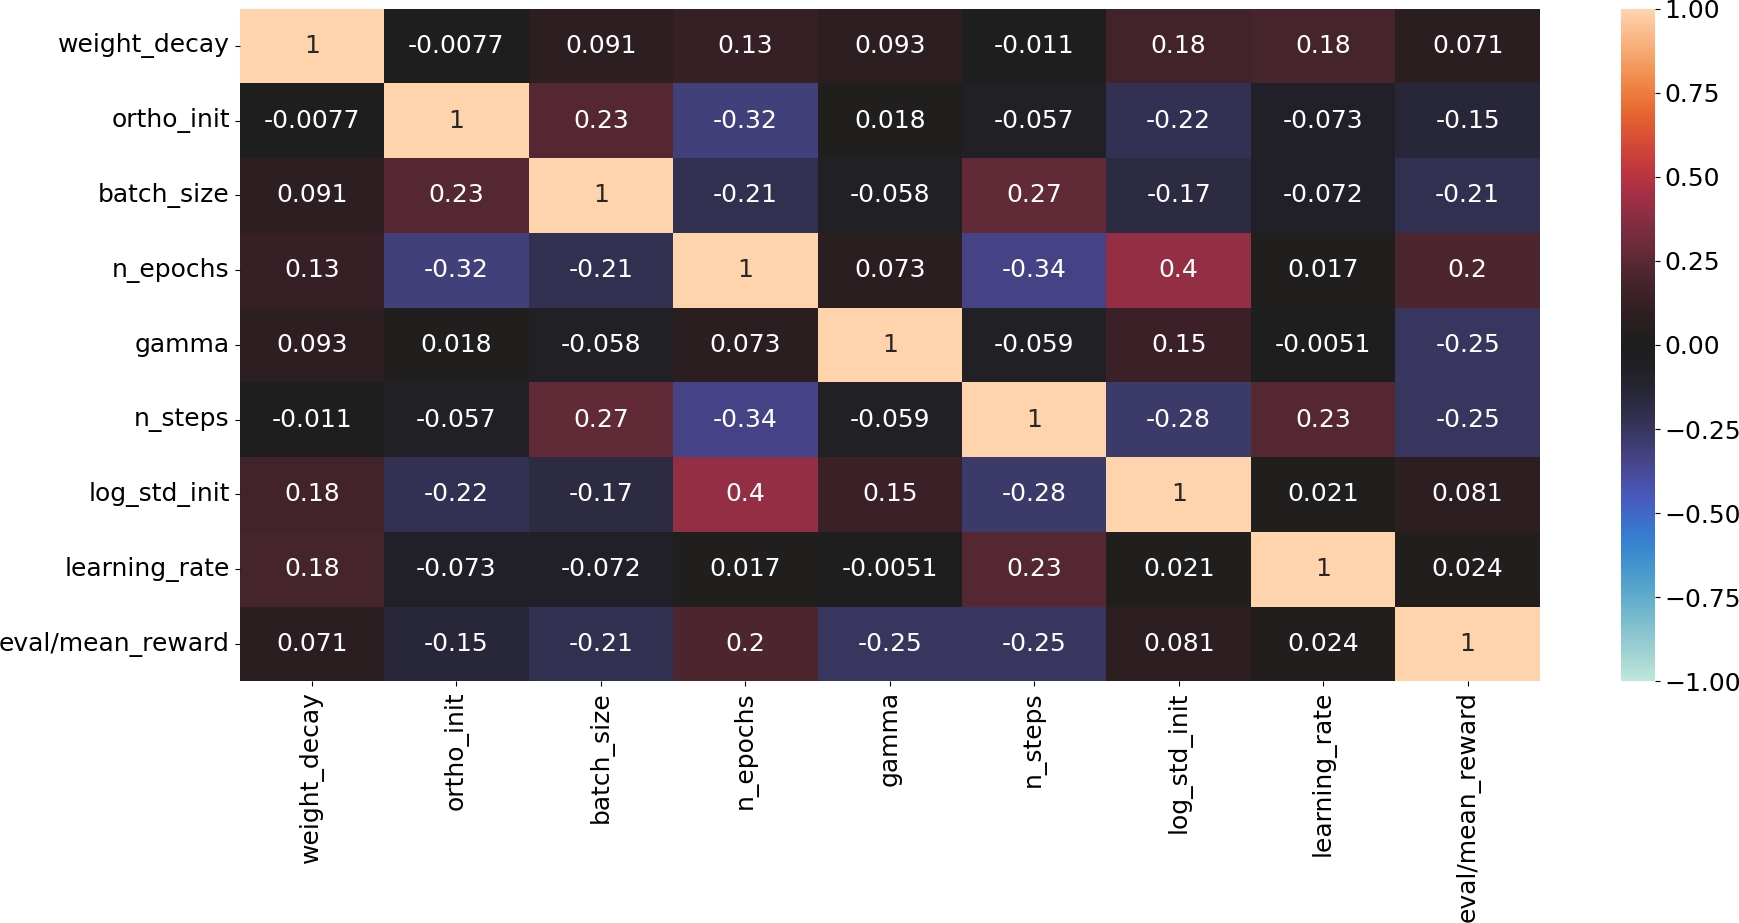}
    \caption{Correlation matrix between hyperparameters and reward}
    \label{fig:corr}
\end{figure*}

\newpage

\subsection{Limitations}

Figure~\ref{fig:lim} illustrates the situation for the index finger when trying to perform the letter "F". We can see that, for each joint of the finger, the reference and simulated positions are very close. Hence, we concluded that the non-similarity between the imitated and reference letter "F" are due to limitations in the tracking algorithm.

\begin{figure*}[ht]
    \centering
    \begin{subfigure}{0.9\textwidth}
        \centering
        \includegraphics[width=0.99\textwidth]{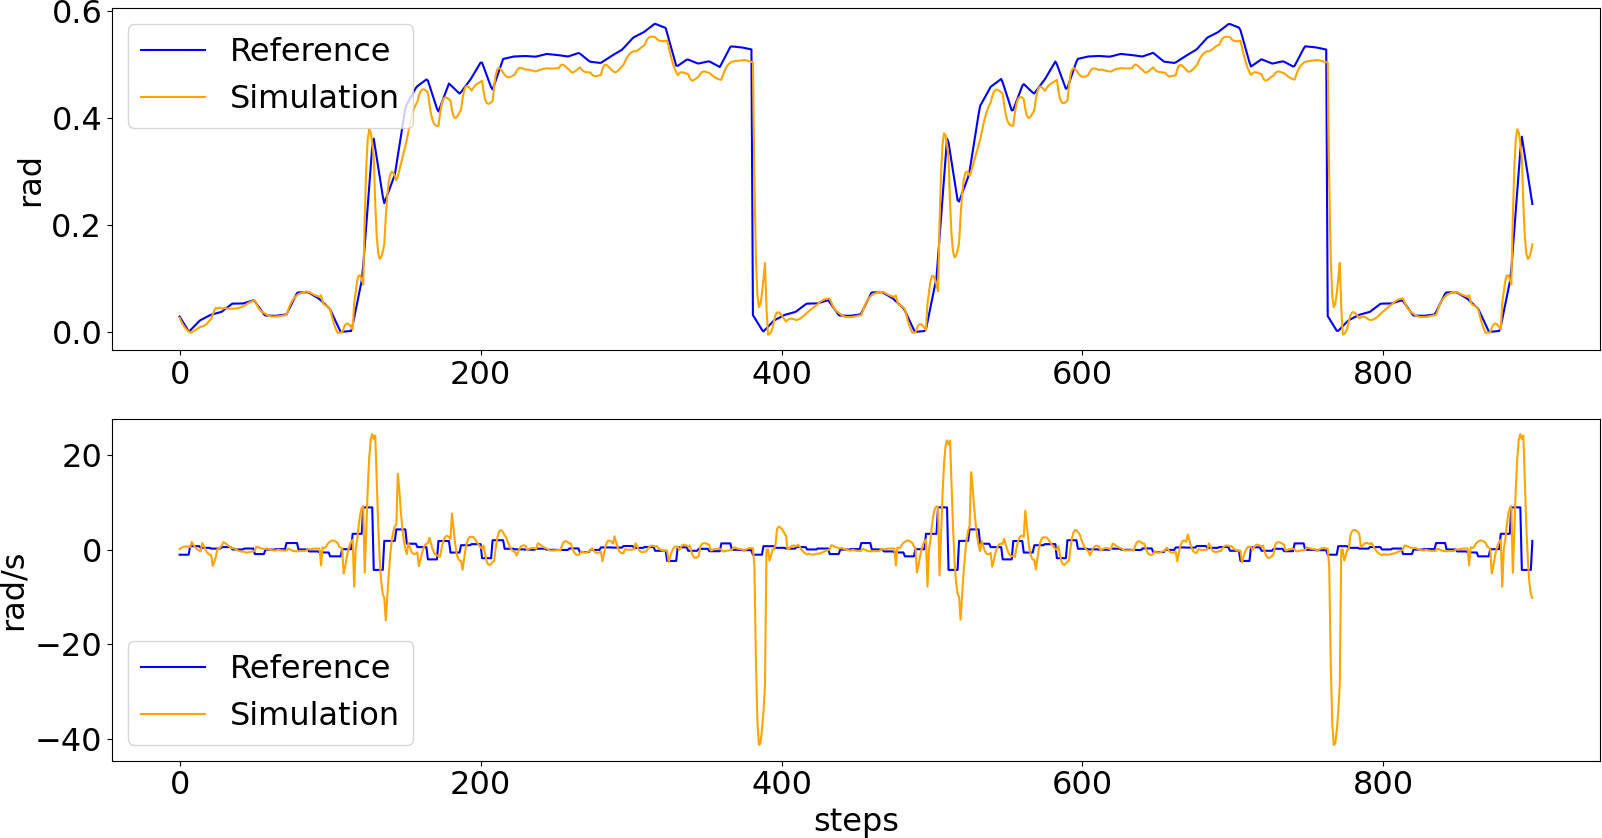}
        \caption{Metacarpophalangeal joint}
        \label{fig:meta}
    \end{subfigure}
    \vfill
    \begin{subfigure}{0.9\textwidth}
        \centering
        \includegraphics[width=0.99\textwidth]{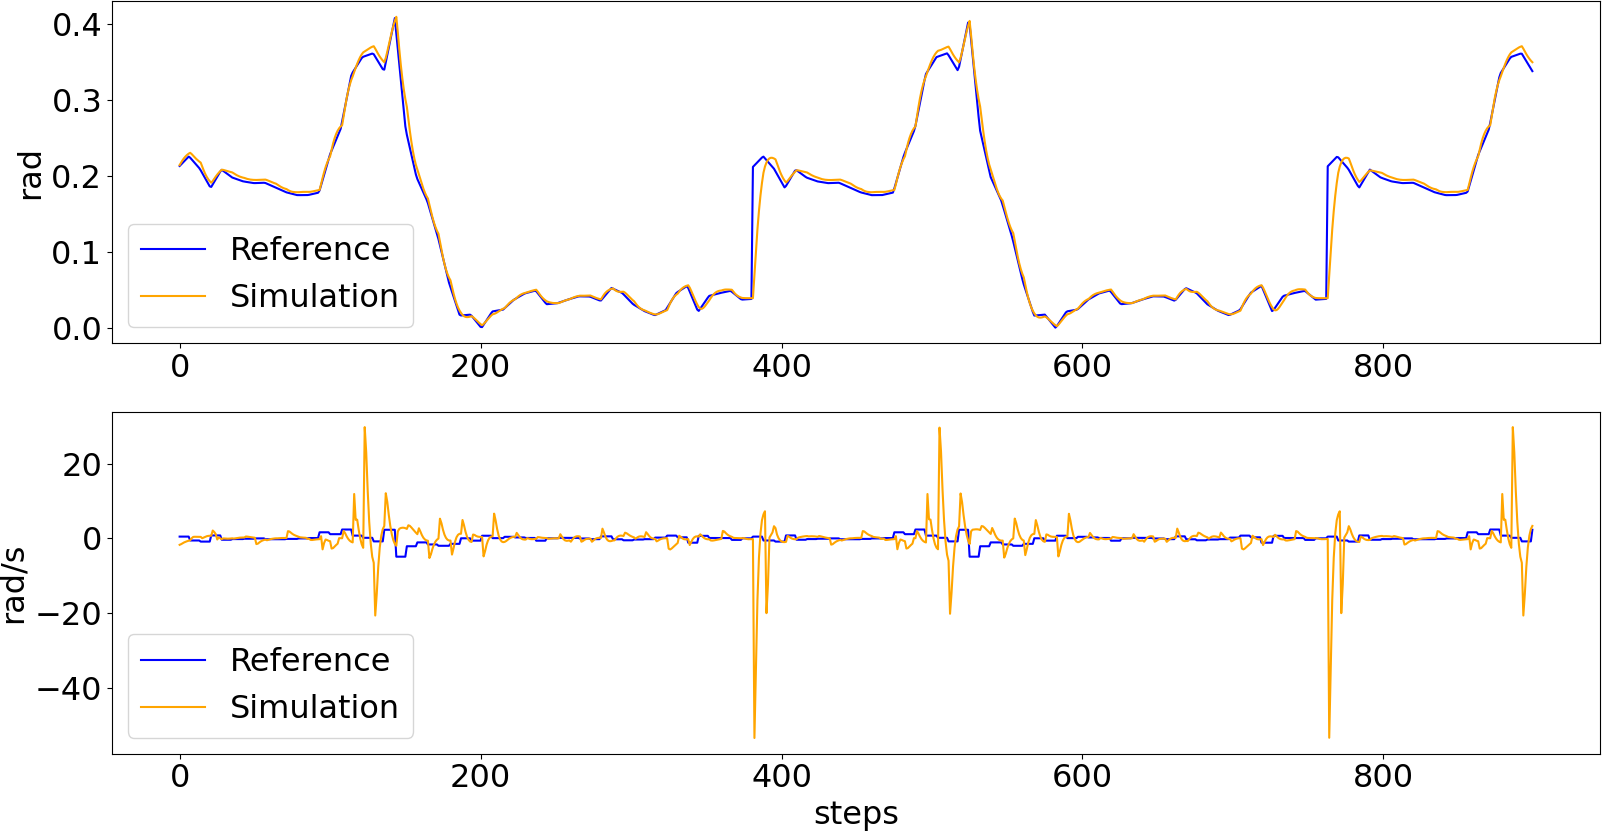}
        \caption{Proximal interphalangeal joint}
        \label{fig:proxi}
    \end{subfigure}
    \vfill
    \begin{subfigure}{0.9\textwidth}
        \centering
        \includegraphics[width=0.99\textwidth]{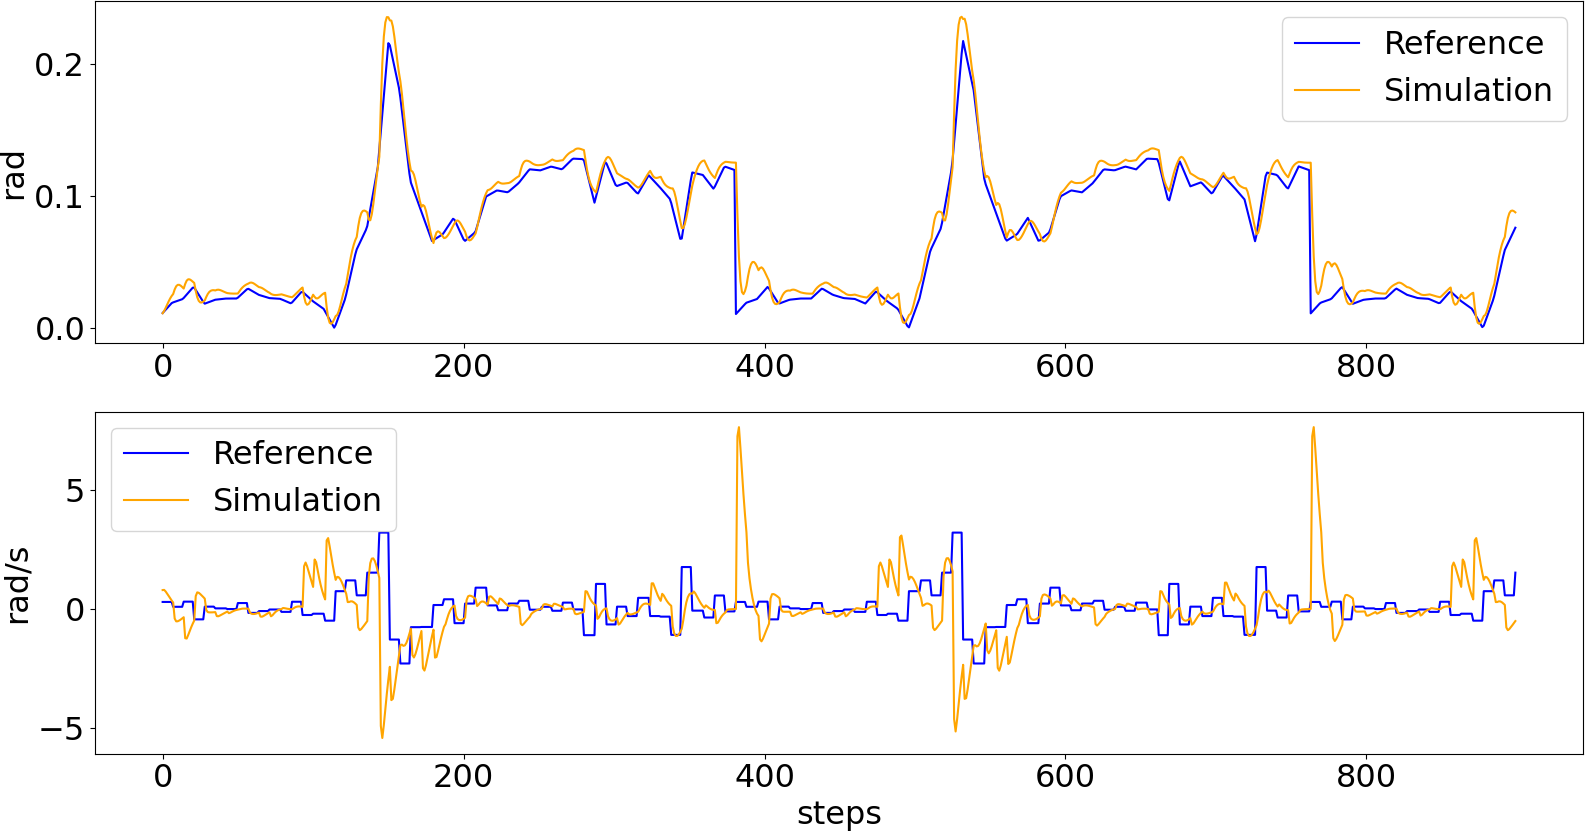}
        \caption{Distal interphalangeal joint}
        \label{fig:dista}
    \end{subfigure}
    \caption{Comparison between the reference and simulated position (left) and velocity (right) of the index finger joints for the motion representing the letter "F"}
    \label{fig:lim}
\end{figure*}
